# Supplementary material for: Few-Shot Text Ranking with Meta Adapted Synthetic Weak Supervision
Source: arXiv:2012.14862 source file (2021-06-02)
Supplement: Supplementary file 1 [file Appendix-0202.tex]

\section{Appendices}

%% *****************************************
%% *****************************************
\subsection{Normalization of Meta-Weights}
\label{sec:appendix:meta}

% Figure~\ref{fig:meta_loop} illustrates the two-step weight calculation process of weak supervision with Meta Learning To Rank (\metaltr{}). Other meta-learning techniques can also be applied in our setting.

% For each mini-batch of weak supervision samples, \metaltr{} first conducts a meta-forward update, which obtains the loss on the synthetic data batch weighted by $w = \{w_j\}_{j=1}^{n}$ and then use the loss to pseudo-update the neural ranker (Eq. \ref{eq:meta-forward}). After the update, the loss on the few-shot target data can be obtained, which is the function of both $\theta$ and $w$. (Figure~\ref{fig:meta_forward}).

% To arrive at our goal of optimizing the weight assignment, we update $w$ using the loss on the target data:

This part elaborates the batch normalization process in Eq. \ref{eq.meta-gradient}.
Following~\citet{ren2018learning}, we set the initial weight $w_j$ to zero and clip negative weights to zero after gradient descent:
{\small
\begin{align}
\tilde{w}_{j} &= - \eta \frac{\partial  }{\partial  (w_j)}  \sum_{i=1}^{m} \frac{1}{m} l_i (\theta^{t+1}(w)), \\
\hat{w}_{j} &= \max (0, \tilde{w}_{j}).
\end{align}
}
We then perform normalization on each minibatch for better stability:
\begin{equation}
    \small
    w_{j}^{*} = \frac{\hat{w}_{j}}{(\sum_{p=1}^n \hat{w}_{p}) + \delta(\sum_{p=1}^n \hat{w}_{p})}
\end{equation}
where $\delta(\sum_{p=1}^n \hat{w}_{p})$, set to prevent division error, takes the value of 1 if $\sum_{p=1}^n \hat{w}_{p} = 0$ and 0 otherwise.
%Note that the denotations are slightly different from what we use in Eq.~\ref{eq.meta-gradient} in order to properly describe the normalization process.

% In practice, the initial weight $w$ is set to zero, presuming an equal importance for all data points in a batch. Also, this approach effectively eliminates the hyperparameter $\eta$.
With this normalization process, the influence of hyperparameter $\eta$ is effectively eliminated. 
The normalization method is not constrained, other approaches can also be used~\cite{shu2019meta, hu2019learning}.

% The meta-gradient can be obtained via automatic gradient calculations in the neural network with deep learning library, such as PyTorch and Tensorflow.
% Intuitively, the meta-gradient reflects the similarity of the weak supervision data and the target few-shot data, and the similarity of the neural networks' gradients on them~\cite{ren2018learning}.

% In practice, the initial weight of $\epsilon$ is set to $0$~\cite{ren2018learning}, so that we can discard the initial weight of $\epsilon$ and directly use the gradient to measure the importance of weak supervision instances (E.q.~\ref{eq.meta-gradient}).


% where $\delta(\sum_{p=1}^n \hat{w}_{p}) = 1$ when $\sum_{p=1}^n \hat{w}_{p} = 0$, to prevent division error, otherwise it is $0$.

% \input{Diagrams/meta_loop}

%% *****************************************
%% *****************************************


\subsection{Supplementary \meta{} Details}
~\label{sec:appendix:implementation}

% \textbf{\meta{}.} This part describes the implementation details of \meta{}, including \textit{Contrastive Synthetic Supervision (\textit{\contrast{}}) Source} and \textit{Meta Learning to Rank}.

% \textit{\contrast{} Source.} We take the small version of T5 (with 60 million parameters) as the NLG model and use MS MARCO as its training source. The maximum input length is set to 512. Optimization uses Adam with a learning rate of 2e-5 and a batch size of 4. During inference, the T5 generator was applied to the target dataset's documents to synthesize large domain-adapted synthetic queries with greedy decoding. The training and inference setups are consistent with the synthetic method form~\cite{ma2020zero} except our contrastive generation strategy.

% \textit{\contrast{} Source.} As mentioned in Sec. \ref{sec:method}, we utilize T5 generator for data synthesis. The generator is trained with approximately 8M triples from MS MARCO, which requires about 60 hours of training time on a single RTX 2080 gpu. 
% In constructing target-domain document pairs, we randomly sample 5 pairs among the top 100 BM25 retrieval results for each seed query $q^*$. The document with higher retrieval score is regarded as the positive document ${d^+}'$ in generation.

% We consider \contrast{} as our ablated baselines that trains neural rankers using contrastive synthetic supervision without \textit{Meta-Learning to Rank.} 

% \textit{Meta-Learning to Rank.} 
This part describes supplementary implementation details of \textit{Meta Learning to Reweight}.
Our model is constructed with deep learning library PyTorch.
We utilize the its automatic differentiation (torch.autograd.grad) to compute the second-order gradient of target loss ($l_i (\theta^{t+1}(w))$) with regard to initial weight ($w_j$) in Eq.~\ref{eq.meta-gradient}. Then the weights are updated and normalized to obtain the reweighted loss, which is later used to train neural rankers.

% In meta-selection,
% We refer to the process of weight assignment for training data as meta-selection, in which we use the contrastive synthetic supervision data as weak supervision data, and the training fold of the target evaluation datasets as few-shot target data. 
% To learn the synthetic data weights, the automatic differentiation (torch.autograd.grad) in PyTorch is used to compute the second-order gradient of the target data loss with respect to initial weights. 

% The parameters of neural rankers are optimized with Adam optimizer, and the learning rate is set to 2e-5.
% We utilize Adam optimizer to optimize the parameters in neural rankers with the learning rate of 2e-5. 
% Both batch size of weak supervision data ($n$) and few-shot target data ($m$) are set to 8. 

% The Meta Learning to Rank (\metaltr{}) process is illustrated in Figure~\ref{fig:meta_loop}. Intuitively, we would optimize the data weights by standard back-propagation from the target in Eq.~\ref{eq:meta}, to parameter $\theta^*$, and then to the data weights $w$ in Eq.~\ref{eq:weak}. 
% The non-trivial part that requires meta-learning is to propagate the gradients through the $\arg\min$ learning operation on $\theta$~\cite{metalearningtutorial, ren2018learning}. As the first step of bringing in recent meta-learning techniques in Few-Shot Neu-IR, \meta{} applies a simple meta-learning method from Ren et al.~\cite{ren2018learning} to complete the loop. Our setting is not restricted to any specific meta-learning methods, and other meta-learning techniques can also be applied~\cite{zheng2019meta, shu2019meta, hu2019learning}.

%% *****************************************
%% *****************************************

\subsection{Supplementary Material for TREC-COVID R5}
~\label{sec:appendix:r5_new_query}

Here we introduce the TREC-COVID R5 task, our results and the implementation details of our methods.

\textit{TREC-COVID R5 Task.} The TREC-COVID Challenge is an ad hoc search task consisting of series of rounds.
The Round 5 we use takes the July 16, 2020 version of CORD-19 dataset as document set, and uses 50 biomedical topics as testing queries. 
The task adopts residual collection evaluation
~\cite{Salton1997ImprovingRP}, which allows the use of relevance labels from previous rounds but will remove all annotated documents before scoring. 

Since the relevance labels of queries from previous rounds (1-45) are available during training, we mainly focus on the results of queries newly created in this round (46-50).
% The document set, topics (queries) set and relevance judgments are all cumulative through the rounds, meaning that the data used in one round is (largely) the superset of data used in the previous round. The task adopt residual collection evaluation, which removes all previously annotated documents before computing scores. The Round 5 we use contains 50 topics (queries), in which the first 45 are from previous rounds and the last 5 are newly created.
\input{Diagrams/r5_new_query} 
\textit{Evaluation Results.}
In Table \ref{tab:r5_new_query}, we show the comparison of our three \meta{} methods and top 10 feedback runs from the official leaderboard. 
It can be seen that our best single model method (\textit{m}) outperforms all other runs, surpassing a leaderboard run by 13.46\% in NDCG@20 score, and 17.50\% in P@20 score. 
% The performance of our fusion method, though slightly lower, is also on par with the best runs on the leaderboard.
This result proves the outstanding generalization ability of our methods. 

It is also noticeable that the performance of top 10 teams on new queries varies greatly (13.41\% NDCG score difference between the best and the worst runs), in contrast to their relatively close performance on all queries (5.06\% NDCG score difference). This discrepancy  confirms our consideration about residual collection evaluation.


% In this part we present the comparison between our results and top feedback runs on TREC-COVID Round 5 leaderboard, in supplement to Sec.~\ref{sec:hybrid}. Due to the incremental nature of this dataset, old queries (1-45) are shared by validation set and test set, which means that their relevance judgments are visible during training. Therefore, we believe that each method is best measured using their performance on new queries (46-50), which can demonstrate their generalization ability on unseen queries. We show the NDCG@20 and P@20 scores of top 10 feedback runs on TREC-COVID R5 leaderboard along with our three settings in Table \ref{tab:r5_new_query}.
\input{Diagrams/appendix_examples}


\textit{Implementation Details.}
This part describes the implementation details of our three method. We first obtain two single models \meta{} (rerank fusion.1) and \meta{} (rerank fusion.2), then fuse them to get \meta{} (RRF).

The general settings of the single-model methods are kept consistent with our methods in Sec. \ref{sec:method}: we use BERT rankers, initialized with PudMedBERT-base, to rerank top 100 results in base retrieval runs from Anserini\footnote{\url{https://github.com/castorini/anserini/blob/master/docs/experiments-covid.md}} (row 7 and 8 for Round 5) respectively.
% The three settings of ours are obtained as follow: \meta{} (rerank fusion.1) and \meta{} (rerank fusion.2) are obtained through a two-stage training, reranking two base retrievals from Anserini\footnote{\url{https://github.com/castorini/anserini/blob/master/docs/experiments-covid.md}} (row 7 and 8 for Round 5) respectively.
For training data, We first use document set of TREC-COVID task to obtain synthetic data with \contrast{}, and then merge it with Medical MARCO (1:1). \meta{} is adopted using the merged data as weak supervision source and relevance labels from previous rounds as target source. After that, the rankers are further trained directly using the relevance labels, with part of the data held out to select the best checkpoints. We adopt Adam optimizer with a learning rate of 2e-5, and set batch size of both synthetic data and target data to 8.

After obtaining the two single-model methods, we adopt reciprocal rank fusion \cite{cormack2009reciprocal} to produce \meta{} (RRF), with $k$ set to 1. The implementation used is from open source library trec-tools \cite{palotti2019}.

What needs to be noted is that NIST has conducted a post-processing to all runs submitted to TREC-COVID R5. To ensure fairness in comparison, we also perform the same post-processing to all our methods.

% Because of a change in document ID that was unaware to participants at Round 5 submission time, all runs submitted are later filtered by NIST to remove documents that were annotated in previous rounds. We obtain the ID mapping from NIST and perform the filtering ourselves, ensuring that our three settings are consistent with those on the leaderboard.

% It can be seen that our best single model method (\textit{m}) surpasses all others in term of new query performance, achieving an NDCG@20 score of 0.8933. The performance of our fusion method, though slightly lower, is also on par with the best runs on the leaderboard. These results prove the outstanding generalization ability of our methods. It is also noticeable that the performance of top 10 teams on new queries varies greatly, despite of their close performance on all queries. 

% This discrepancy suggest that the residual collection evaluation may somehow be biased, and its effectiveness is thus a problem worth the attention of the community.

% 分三个小标题: 1. TREC-COVID R5 setting; 2. evaluation result and analyses; 3. implementation details
% comparison result放implementation details前面
% R5介绍要精简（现在第一段的长度）
% post procession in open source


%%. =1*****************************************
%% *****************************************

\subsection{Supplementary Case Study}
~\label{sec:appendix:case_study}

In Table~\ref{tab:appendix_case}, we provide more cases from the other two datasets, Robust04 and TREC-COVID, to further verify the effectiveness of our weak supervision training framework on few-shot Neu-IR in different domains. The first three cases are from Robust04, and the rest are from TREC-COVID.

For the first case, \contrast{} can extract salient keywords more related to the document topic, such as ``radars'' and ``colombia'' to generate more informative queries, while \QG{} tends to extract general keywords, damaging the correlation between the generated query and the specific document. Besides extracting topical keywords, \contrast{} can also extract some necessary themes from the given document, such as the particular time ``1993'' and the adjective word ``increased'' in the second case. Such a strong keyword extraction ability helps generate an informative and related query for the given document.


The effectiveness of \contrast{} is also shown on the biomedical corpus. \contrast{} captures ``lung'' and ``quarantine prevent'' instead of general keywords such as ``sars cov'' and ``symptoms'', which apparently will appear in many related documents.
%It is evident that ``sars cov'' and ``symptoms'' can be mentioned numerous times in the literature about COVID-19 and matched with many other documents. 
These observations effectively verify that \contrast{} can generate more characteristic and informative queries, synthesizing high-quality weak supervision data for different domains.


We further explore those cases that are assigned zero weights by \metaltr{}, such as the third and the sixth cases. 
% In the third case, the positive document's main topic is political news, rather than the language of the program host, Osvaldo Rodriguez. 
In the third case, \contrast{} constructs the query with keywords ''language'' and ''osvaldo rodrigrez'', which are in fact irrelevant in the original document, altering the query off-topic.
% \metaltr{} shows its effectiveness in filtering such mismatched query-document pairs. 
%For the sixth case, the two documents are both related to the query ``covid-19 pandemic effects on society''. 
For the sixth case, \contrast{} fails to exclude the phrase ''covid-19 pandemic'' which is shared by both documents. Therefore, the synthesized query is indistinguishable.
% Fortunately, \metaltr{} can effectively identify such multi-document matched instances to avoid the misleading from the noisy training signals.
Fortunately, \metaltr{} can effectively identify such instances where the match between query and positive document is not clear and unique, and preclude the misleading noisy signals by assigning them zero meta-weights.



% Besides extracting topical keywords, ContrastQG can also extract some necessary themes from the given document documents, such as the particular time "1993" and adjective word ``increased'' in the second case. Such strong ability of keyword extraction helps to generate an informative and related queries for the given document.

% In Table~\ref{tab:appendix_case}, we supplement more cases selected by \meta{} on the other two datasets, Robust04 and TREC-COVID. The first 3 cases are from Robust04, and the last 3 cases are from TREC-COVID. The former’s documents are news articles, while the latter’s are biomedical literature on COVID-19.
% In these samples selected by \meta{}, the query generated by ContrastQG indeed captures the specific content of positive documents that are different from negative documents and contains richer and more specific information. These results are consistent with our observations for ClueWeb09-B in Sec.~\ref{sec:case_study}. 


% Here we show more cases of synthetic queries that are assigned positive weights by \meta{}. Case 1-3 in Table \ref{tab:appendix_case} are selected from Robust04 and Case 4-6 are selected from TREC-COVID. Consistent with our observation in ClueWeb09-B, ContrastQG is able to capture the difference between two documents, while QG tends to extract keywords and generate general contents.
