# Supplementary material for: Few-Shot Text Ranking with Meta Adapted Synthetic Weak Supervision
Source: arXiv:2012.14862 source file (2021-06-02)
Supplement: Supplementary file 2 [file old_Appendix.tex]

\section{Appendices}

%% *****************************************
%% *****************************************
\subsection{Learning to Weight by Meta-Gradients}
~\label{sec:appendix:meta}

Intuitively, we would optimize the data weights by standard back-propagation from the target in Eq.~\ref{eq:meta}, to parameter $\theta^*$, and then to the data weights $w$ in Eq.~\ref{eq:weak}. 
The non-trivial part that requires meta-learning is to propagate the gradients through the $\arg\min$ learning operation on $\theta$~\cite{metalearningtutorial, ren2018learning}. As the first step of bringing in recent meta-learning techniques in Few-Shot Neu-IR, \meta{} applies a simple meta-learning method from Ren et al.~\cite{ren2018learning} to complete the loop. Our setting is not restricted to any specific meta-learning methods, and other meta-learning techniques can also be applied~\cite{zheng2019meta, shu2019meta, hu2019learning}.



% The meta-learning process is illustrated in Figure~\ref{fig:model_outline}.

% The main idea is that, 
For each weak supervision mini-batch, \meta{} first conducts a meta-forward loop, including updating the neural ranker using a weakly supervised batch (Eq.~\ref{eq:weak}) and calculating the new few-shot target loss (Eq.~\ref{eq:meta}). The goal is to construct a computing graph of the weak supervision process, on which the meta-gradients can be obtained using the automatic gradient calculation on the neural network.

Specifically, at the $t$-th training step, we first assign some random weights $\epsilon$ on the training signal in the weak supervision batch:
\begin{align}
    L' (\theta^t; \epsilon) =  \sum_{j=1}^n \epsilon_j l'_j(\theta^t).
\end{align}
Then we conduct standard updates on this weak supervision batch using the gradients\footnote{The derivation described here uses vanilla SGD. Other optimizers can be used.}:
\begin{align}
    \theta^{t+1}(\epsilon)  = \theta^{t} - \alpha  \triangledown \sum_{j=1}^n \epsilon_j l'_j(\theta^t),
\end{align}
where $\alpha$ is the learning rate. 
The updated $\theta^{t+1}$ is used to calculate the ranking loss on a target few-shot batch:
\begin{align}
    L(\theta^{t+1}(\epsilon)) &= \sum_{i=1}^m l_i(\theta^{t+1}(\epsilon)),
\end{align}
and our goal is to find the optimized training weights  $\epsilon^{*}$:
\begin{align}
    \epsilon^{*} = \arg\min_{\epsilon}  L(\theta^{t+1}(\epsilon)). \label{eq:metaloss}
\end{align}
According to Eq.~\ref{eq:metaloss}, the data weights can be updated using its meta-gradient:
\begin{align}
    \epsilon^{*}_{j} =  \epsilon_j - \eta \frac{\partial  }{\partial  (\epsilon_j)}  \sum_{i=1}^{m} l_i (\theta^{t+1}(\epsilon)). \label{eq.meta-gradient}
\end{align}
In practice, the initial weight $\epsilon$ is set to $0$~\cite{ren2018learning}, for a uniform prior on the data quality. This meta-gradient can be obtained via automatic gradient calculations in the neural network, without requiring the exact form, which can be complex for deep neural networks.
In simpler cases such as linear models, Ren et al.~\cite{ren2018learning} showed that the meta-gradient is composed by the similarity of the weak supervision data and the target few-shot data, and the similarity of the neural networks' gradients on them~\cite{ren2018learning}.

We clip negative meta-gradients to zero as it is unlikely a weak supervision label is ``reversed''. Most time it is noise to be ignored. We also normalize the weights in batch for better stability:
% In addition, it is also more stable to keep data weights normalized. Putting these together, the data weights of this weak supervision batch are calculated as:
\begin{align}
w_{j} &= \frac{\hat{w}_{j}}{(\sum_{p=1}^n \hat{w}_{p}) + \delta(\sum_{p=1}^n \hat{w}_{p})},\\ 
\hat{w}_{j} &= \max (0, \epsilon^{*}_{j}).
\end{align}
Here $\delta(\sum_{p=1}^n \hat{w}_{p}) = 1$ when $\sum_{p=1}^n \hat{w}_{p} = 0$, to prevent division error, otherwise it is $0$. 



\input{Diagrams/query_num}
\input{Diagrams/rank_robust}

\subsection{Effectiveness and Efficiency in Fewer Shot}
~\label{sec:appendix:meta_analysis}
This experiment investigates the behavior of selective weak supervision methods with different amounts of few-shot labels. 
We randomly select one testing split of ClueWeb09-B, vary the number of queries in the few-shot training target, and evaluate the performance of \meta{} and ReInfoSelect with the same weak supervision data. The results are shown in Figure~\ref{fig:few_shot}. 

In Figure~\ref{fig:query_num}, the accuracy of all few-shot rankers grows with more target labels. Conv-KNRM benefits more with more relevance labels than BERT as the latter is pretrained. With \meta{}, as few as 20 labeled queries are needed for BERT Ranker to improve SDM. 
This amount of manual relevance labels is feasible to obtain in many real-world scenarios. In contrast, though also benefits from more labels, ReInfoSelect never elevates either neural rankers to outperform their base retrieval (SDM), even with all available training queries.

Especially with BERT-style enormous models, training efficiency is another important factor to consider in selective weak supervision, where we exchange some efficiency overhead in data selection for better few-shot accuracy.
Figure~B shows this overhead by comparing the training efficiency of weak supervision with and without data selection.
{\meta{}} spends a 2.5 times efficiency overhead in constructing the meta forward loop and then the meta-gradient (Figure~C). The overhead cost is constant to the few-shot label amount and model complexity. 
% (Figure~\ref{fig:model_outline})
In comparison, ReInfoSelect raises a dilemma in trading off efficiency-effectiveness: its policy gradient can provide better weak supervision guidance with more target labels where the reward is more stable, but the cost of calculating rewards grow dramatically with more target labels. 
The trial-and-error mechanism in reinforcement learning is more costly than meta-gradients even with only 10 target queries.

We also plot the few-shot accuracy at different learning steps in Figure~\ref{fig:bert_rb}. As shown in the comparison, BERT ranker trained with {\meta{}} behave more stably. In comparison, ReInfoSelect requires warming up the neural rankers with the trained weights of {All Anchor}, otherwise (in our experiment) it does not converge well. Still, after warming up, ReInfoSelect only slightly boosts the ranking accuracy in the beginning and starts to overfit quickly.

% \input{Diagrams/meta_case_examples}
\input{Diagrams/appendix_examples}

\subsection{Case Studies}
~\label{sec:appendix:case_study}
In this last experiment, we quantitatively investigate the data selection behavior of ReInfoSelect and {\meta{}}. Using the same ClueWeb09 target fold and BERT Ranker, We randomly pick a batch of anchor data, inject it at different steps of weakly supervised learning, and collect its assigned weights for manual examination.  Some examples are listed in Table~\ref{tab:case}.

Even when the BERT Ranker is near convergence and the optimization becomes more sophisticated, {\meta{}} still selects high-quality weak supervision signals for it. 
In Table~\ref{tab:case}, anchor-documents received positive meta-gradient (top half) are very legitimate relevance-alike signals: The anchor texts perhaps have been used as actual web search queries; the positive documents are indeed relevant and the negative ones are not.
In comparison, those received negative meta-gradient (bottom half) include variant types of noises. Neither pseudo positive nor negative documents for Case 5, 6, and 8 are relevant. They are all discarded by \meta{}.
% } learns to discard them as they provide no useful signal.
Case 7 is a more dangerous distraction. Its pseudo positive document is irrelevant but the pseudo negative document from BM25 is actually relevant. Without effective selection, this weak supervision signal may even move the neural ranker to the wrong direction and completely disturb the model learning. More examples will be included in our open-source repository.
% to help understand why using meta-gradients to select weak supervision signals is effective.
