# Supplementary material for: Few-Shot Text Ranking with Meta Adapted Synthetic Weak Supervision
Source: arXiv:2012.14862 source file (2021-06-02)
Supplement: Supplementary file 3 [file old_appendix_examples.tex]

\begin{table*}[t]
\centering
\small
\scalebox{0.93}{
\begin{tabularx}{\textwidth}{lX|X|X}
  \toprule
  \multicolumn{2}{l|}{\textbf{Synthetic Query}} & \textbf{Positive Document} & \textbf{Negative Document} \\ 
    \multirow{2}{*}{(1)} &
    \texttt{ContrastQG:} why did the us \redbf{boycott} cuba
    \newline
    \texttt{QG:} who violated the \bluebf{embargo} on cuba
    & 
    … attempt to present the U.S. \redbf{boycott} as a  blockade,' an  \bluebf{embargo},' or a sort of  sanitary cordon' that is virtually driving Cuba to famine. \  The United States has placed Cuba under a trade \redbf{boycott}...
    & 
    … Mr Ernest Preeg, former chief economist at the US Agency for International Development and author of a recent study on Cuba's economic prospects once the US trade \bluebf{embargo} is lifted ... 
    \\
    \hline
    \multirow{2}{*}{(2)} &
    \texttt{ContrastQG:} us military \redbf{radars} in \redbf{colombia} 
    \newline
    \texttt{QG:} what is the \bluebf{pentagon}
    & 
    …  One month ago, the \bluebf{Pentagon} issued an order to suspend operations of the two \redbf{radars} that detect aircraft. These \redbf{radars} operate in \redbf{Colombia} as a result of that agreement. ...
    & 
    ...  provide for more funding and retain more forces than the \$1.5-trillion five-year budget Cheney presented to Congress in January, \bluebf{Pentagon} officials say ...
    \\
    \hline
    \multirow{2}{*}{(3)} &
    \texttt{ContrastQG:} what percent of the economy was \redbf{increased} in \redbf{1993}
    \newline
    \texttt{QG:} what is the economic issue in \bluebf{peru}
    & 
    ... This letter explains the \bluebf{Peruvian} Government's economic policy. \  The development of the economy in \redbf{1993} was in general much better. \  It is estimated that the real GDP has \redbf{increased} by 7 percent  ...
    & 
    ... Only three economies - Guyana, Argentina and \bluebf{Peru} - grew by more than than 5 per cent this year, with \bluebf{Peru} expanding by 11 per cent...
    \\
    \hline
    \hline
    \multirow{2}{*}{(4)} &
    \texttt{ContrastQG:} how is \redbf{influenza} transmitted through humans
    \newline
    \texttt{QG:} what \bluebf{pathogens} are transmitted by rats
    & 
    Animal Models for \redbf{Influenza} Virus \bluebf{Pathogenesis} and Transmission \redbf{Influenza} virus infection of humans results in a respiratory disease ...
    & 
    ... It has been well established that human \bluebf{pathogenic} viruses may be transmitted \  factors that could play a role in the survival of human \bluebf{pathogenic} viruses in ...
    \\
    \hline
    \multirow{2}{*}{(5)} &
    \texttt{ContrastQG:} what were the characteristics of \redbf{covid pneumonia}
    \newline
    \texttt{QG:} can procalcitonin cause \bluebf{influenza}
    & 
    Comparison of Hospitalized Patients with \redbf{pneumonia} caused by \redbf{COVID}-19 and \bluebf{influenza} Since the outbreak of Coronavirus Disease 2019 (\redbf{COVID}-19) \  differentiate \redbf{COVID}-19 from other respiratory infectious diseases, such as \bluebf{influenza} ...
    & 
    The role of animal reservoirs in social-environmental landscapes: remarks on the control of avian \bluebf{influenza} and preparedness for pandemics. \bluebf{Influenza} viruses are well known for their ability to infect and cause disease  ...
    \\
    \hline
    \multirow{2}{*}{(6)} &
    \texttt{ContrastQG:} which receptors are expressed in the human \redbf{lung}
    \newline
    \texttt{QG:} what is \bluebf{sars cov} receptor
    & 
     RESULTS Both \bluebf{SARS-CoV} receptors of ACE2 and CD209L were expressed in the 8 organ/tissue-derived endothelial cells. The expression of ACE2 receptor was the highest in the human \redbf{lung} microvascular endothelial cells, and lowest...
    & 
    ... 2019 novel coronavirus (2019-n\bluebf{CoV})The outbreaks of 2002/2003 \bluebf{SARS}, 2012/2015 MERS and 2019/2020 Wuhan respiratory syndrome clearly indicate that genome evolution of an animal coronavirus (\bluebf{CoV}) may enable ...
    \\
    \bottomrule
\end{tabularx}
}
\caption{The synthetic weak supervision signals selected by \meta{}, where Case 1-3 targets Robust04 and Case 4-6 targets TREC-COVID. The \bluebf{blue} texts are shared by the two documents, and the \redbf{red} texts are the specific content of the positive document. The document snippets are manually selected.\label{tab:appendix_case}
}
\end{table*}


% of \textbf{Robust04}(Case 1-3) and \textbf{TREC-COVID} (Case 4-6).
